# Supplementary material for: Growth optimization of TaN for superconducting spintronics
Source: arXiv:2102.09018 ancillary file (2021-02-17)
Supplement: Supplementary file 1 [file Supplementary_Material.pdf]

# Growth optimization of TaN for superconducting spintronics

M. Müller,[1,2,a)] R. Hoepfl,[1,2] L. Liensberger,[1,2] S. Geprägs,[1] H. Huebl,[1,2,3] M. Weiler,[4,1,2] R. Gross,[1,2,3] and M. Althammer[1,2,b)]
[1)] *Walther-Meißner-Institut, Bayerische Akademie der Wissenschaften, 85748 Garching, Germany*
[2)] *Physik-Department, Technische Universität München, 85748 Garching, Germany*
[3)] *Munich Center for Quantum Science and Technology (MCQST), Schellingstraße 4, 80799 München, Germany*
[4)] *Fachbereich Physik and Landesforschungszentrum OPTIMAS, Technische Universität Kaiserslautern, 67663 Kaiserslautern, Germany*

(Dated: February 17, 2021)

## I. ATOMIC FORCE MICROSCOPY SCANS

Fig. S1 shows exemplary atomic force microscopy (AFM) scans for (a) a plain TaN-film deposited using the following sputter parameters: $N_2$/Ar=0.35, $T_{\mathrm{depo}} = 500°\mathrm{C}$, $p_{\mathrm{depo}} = 5\ \mu\mathrm{bar}$ and $P_{\mathrm{depo}} = 30$ W and (b) the TaN/Py-bilayer (sample A from the main text). The TaN layer of this sample is fabricated using the same optimal deposition parameters, which results in a $T_{\mathrm{c}} = 4.7$ K. The Py layer is deposited at RT using an Ar-atmosphere at $p_{\mathrm{depo}} = 5\ \mu\mathrm{bar}$ for Py using $P^{\mathrm{Py}}_{\mathrm{depo}} = 70$ W. To prevent oxidation of the samples a Ta-capping layer is deposited at RT and $p_{\mathrm{depo}} = 5\ \mu\mathrm{bar}$ using $P^{\mathrm{Ta}}_{\mathrm{depo}} = 30$ W. The observed RMS (root mean square) roughness is below detection limit ($< 300$ pm) for our samples.

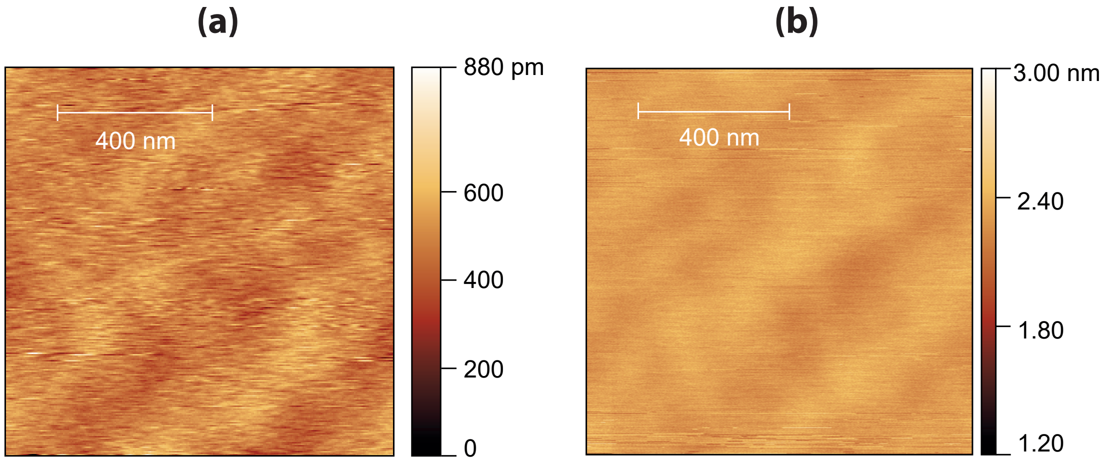


Figure S1. Atomic force microscopy (AFM) roughness scans of a 1 $\mu m^2$-area for a plain TaN-film (a) and the TaN/Py-bilayer (b). The extracted RMS surface roughnesses are 60 pm (a) and 70 pm (b), respectively.

a) manuel.mueller@wmi.badw.de
b) matthias.althammer@wmi.badw.de

## II. S2.ADDITIONAL GROWTH OPTIMIZATION PARAMETERS

Additional optimized sputter deposition parameters are shown in Fig. S2.

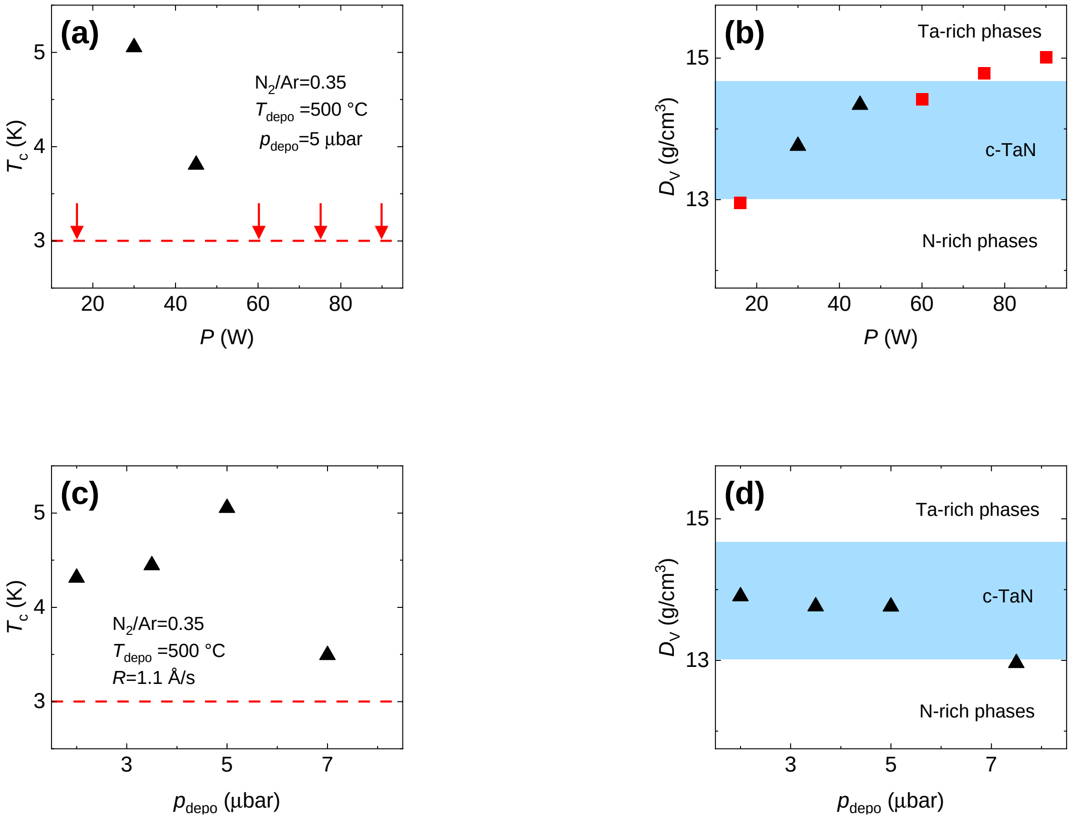


Figure S2. Superconducting transition temperature $T_c$ (a) and material density $D_V$ (b) of the TaN thin films as function of the deposition power $P_{depo}$. (c), (d), we plot $T_c$ and $D_V$ as function of the deposition pressure $p_{depo}$. Samples that did not exhibit full superconductivity above $T = 3$ K are represented by red vertical arrows at $T = 3$ K in (a) as well as red squares in (b).

In Fig. S2(a), we plot the superconducting transition temperature $T_c$ as function of the deposition power applied for our 3 inch Ta-target. For the used $N_2$/Ar-flow ratio of 0.35, we observed only two SC films with a $T_c > 3$ K for intermediate powers. The volume density $D_V$ of these two films in Fig. S2(b) is situated within the expected density range for cubic TaN. For rising deposition powers, we observe a rise in $D_V$.
For the superconducting $T_c$ and volume density $D_V$ as a function of deposition pressure in Fig. S2(c),(d), we observe nearly constant values for low pressures and a reduction in $T_c$ and $D_V$ for higher deposition pressures.

## III. TANTALUM NITRIDE WITH OPTIMIZED RECIPE ON SAPPHIRE SUBSTRATE

As a test, we use the optimized recipe for the growth of TaN (sputter parameters:$N_2$/Ar=0.35, $T_{\rm depo} = 500°$C, $p_{\rm depo} = 5\ \mu$bar and $P_{\rm depo} = 30$ W) on a c-plane $Al_2O_3$ (sapphire) substrate and performed Van-der-Pauw-transport as well as x-ray diffraction experiments to determine both the superconducting transition temperature $T_{\rm c}$ and the crystalline quality of the TaN thin film.

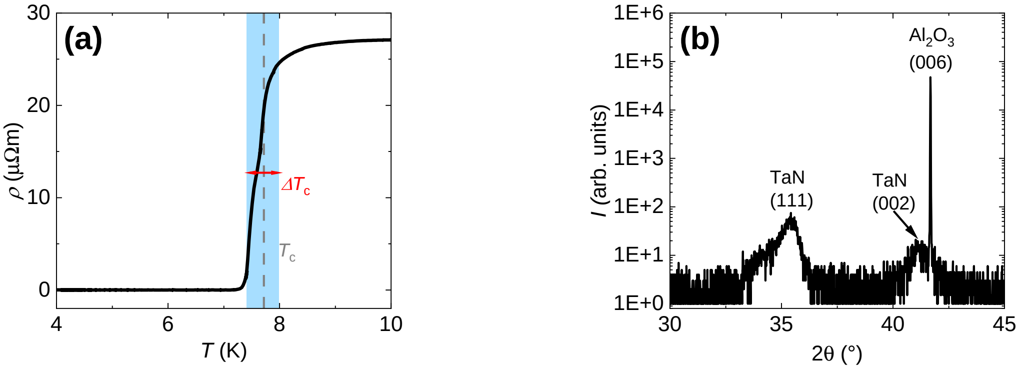


Figure S3. Resistive transition behavior $\rho(T)$ (a) and x-ray-diffraction pattern (b) of a 60 nm thick TaN film grown on a c-plane $Al_2O_3$-substrate.

In Fig. S3(a), we plot the resistivity as a function of temperature $\rho(T)$ of the TaN film grown on a c-plane $Al_2O_3$ substrate. It exhibits a superconducting transition temperature of $T_{\rm c} = 7.72$ K, which is almost 3 K higher than that of TaN grown on $SiO_2$. In Fig. S3(b), we can clearly see the (111)- and (002)-reflections of cubic TaN in the x-ray diffraction $2\theta$-$\omega$-scan in agreement with Refs. 1 and 2.

## IV. X-RAY REFLECTOMETRY ON SC/FM-BILAYER

The results of the performed x-ray reflectometry are shown in Fig. S4 for sample A and B of the main text with the fitted simulation curve using Leptos$^{TM}$.

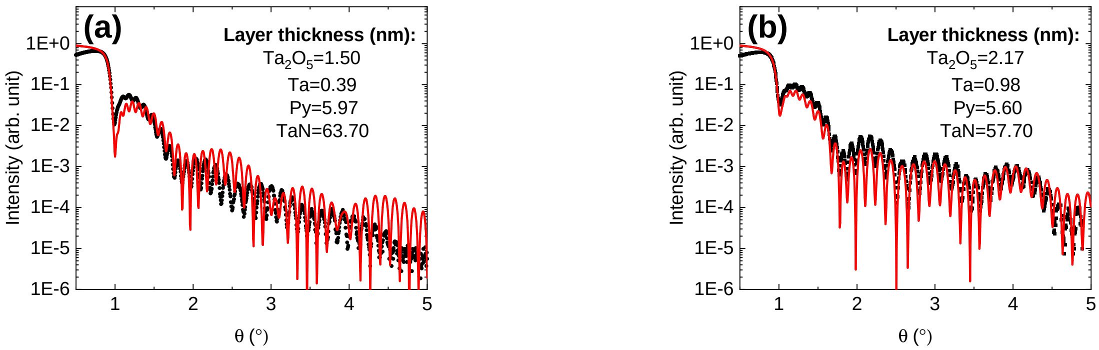


Figure S4. X-ray reflectometry of the two TaN/Py-bilayers with TaN grown in (a) the superconducting state (sample A) and (b) the normal state (sample B). The extracted thickness of the respective layers is given in the insets.

The used densities of the individual materials for fitting are listed in Tab. S1.

| Material | NC TaN | SC TaN | Py | Ta | $TaO_x$ |
|---|---|---|---|---|---|
| Density ($g/cm^3$) | 15.5 | 13.7 | 8.7 | 14.5 | 7.5 |

Table S1. Used densities for the individual materials for the fitting curves in Fig. S3.

The variations in density between the NC- and SC-TaN are due to the formation of different TaN-compounds in agreement with Fig. 1(d) of the main text.

## V. MAGNETIZATION DYNAMICS PARAMETERS OF THE SC/FM-BILAYERS

In the following two sections, we will provide a step by step instruction on how we extract both the magnetization dynamics parameters and inverse current-induced torques $\sigma^{\mathrm{SOT}}$ out of our raw $S_{21}(\mu_0 H_{\mathrm{ext}})$-data. This data analysis procedure is equal to the one derived in our previous work[3] and is provided here to support the establishing of this method for other groups performing bbFMR.

The raw $S_{21}(\mu_0 H_{\mathrm{ext}})$ can be expressed as

$$S_{21}(H_{\mathrm{ext}})|_f = C_0 + C_1 \cdot H_{\mathrm{ext}} - iAe^{i\phi} \cdot \frac{\chi_{\mathrm{yy}}(H_{\mathrm{ext}}) + \chi_{\mathrm{zz}}(H_{\mathrm{ext}})}{\mu_0 M_{\mathrm{s}}}, \tag{S1}$$

where $A$ is the resonance amplitude, $\phi$ is the resonance phase, $\mu_0$ is the vacuum permeability and $M_{\mathrm{s}}$ is the saturation magnetization. The $\chi_{\mathrm{ii}}$ are components of the Polder susceptibility tensor. To account for the background $S_{21}^0$, we add a linear function $S_{21}^0 = C_0 + C_1 H_{\mathrm{ext}}$ to Eq. (S1) with the complex offset $C_0$ and slope $C_1$.
For the in-plane Polder susceptibility, we use the following expression[3]:

$$\hat{\chi}_{\mathrm{P}} = \begin{pmatrix} \chi_{\mathrm{yy}} & \chi_{\mathrm{yz}} \\ \chi_{\mathrm{zy}} & \chi_{\mathrm{zz}} \end{pmatrix} = \frac{\mu_0 M_{\mathrm{s}}}{D} \begin{pmatrix} H_{\mathrm{ext}} + H_{\mathrm{ani}} + i\frac{\Delta H}{2} & +\frac{i\omega}{\mu_0\gamma} \\ -\frac{i\omega}{\mu_0\gamma} & H_{\mathrm{ext}} + M_{\mathrm{s}} + H_{\mathrm{ani}} + i\frac{\Delta H}{2} \end{pmatrix}$$
$$D = \left(H_{\mathrm{ext}} + M_{\mathrm{s}} + H_{\mathrm{ani}} + i\frac{\Delta H}{2}\right)\left(H_{\mathrm{ext}} + H_{\mathrm{ani}} + i\frac{\Delta H}{2}\right) - \left(\frac{\omega}{\mu_0\gamma}\right)^2 \tag{S2}$$

The background-corrected change in transmission caused by the sample $\Delta S_{21}$ is defined as[3,4]

$$\Delta S_{21} = \frac{S_{21} - S_{21}^0}{S_{21}^0}. \tag{S3}$$

In Fig. S5, we plot exemplary $\Delta S_{21}(H_{\mathrm{ext}})$-data for sample A from the main text, recorded at $f = 15$ GHz, in the normal- and superconducting state in real (a) and imaginary part (b), respectively.

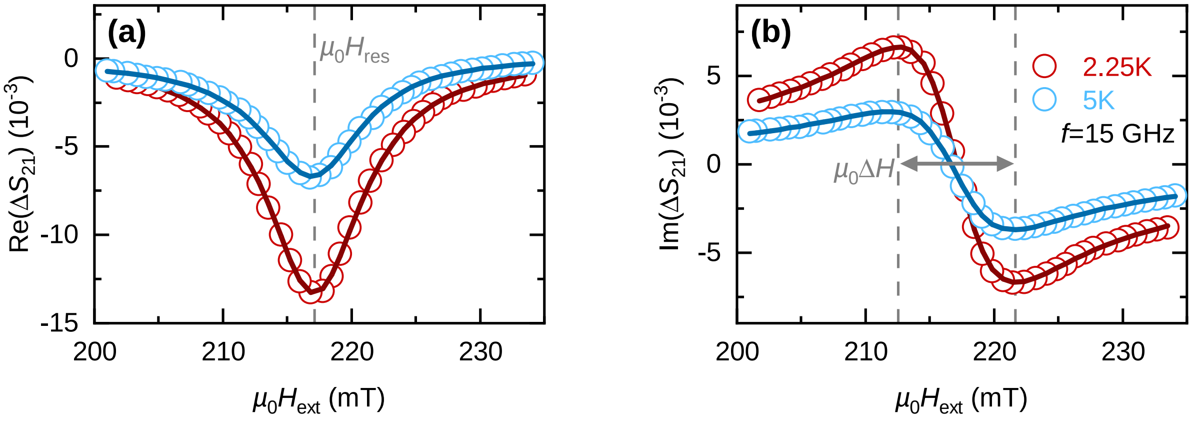


Figure S5. Real (a) and imaginary (b) part of the background-corrected change in transmission $\Delta S_{21}$ for sample A of the main manuscript as a function of external field $\mu_0 H_{\mathrm{ext}}$ at $f = 15$ GHz for temperatures above ($T = 5$ K) and below $T_{\mathrm{c}}$ ($T = 2.25$ K). The lines represent fitting curves following Eq. (S4).

In Fig. S5, we observe the typical complex Lorentzian behavior in $\Delta S_{21}(H_{\mathrm{ext}})$, that can be fitted with

$$\Delta S_{21} = \frac{S_{21} - S_{21}^0}{S_{21}^0} = -i\frac{Ae^{i\phi}}{C_0 + C_1 H_{\mathrm{ext}}} \frac{[\chi_{\mathrm{yy}}(\omega, H_{\mathrm{ext}}) + \chi_{\mathrm{zz}}(\omega, H_{\mathrm{ext}})]}{\mu_0 M_{\mathrm{s}}}. \tag{S4}$$

to extract the FMR-field $\mu_0 H_{\mathrm{res}}$ and -linewidth $\mu_0 \Delta H$, which are analyzed as function of $f$ to obtain the magnetization dynamics parameters. From Fig. S5, it becomes apparent, that the FMR-amplitude $A$ and phase $\phi$ are also greatly affected by the SC transition. These two quantities are a measure of the inductive coupling $L$ between sample and

CPW and are studied as function of $f$ to obtain the $\sigma^{\rm SOT}$ in section VI.
In Fig. S6, we plot the resonance-field $\mu_0 H_{\rm res}$ (a) and the resonance linewidth $\mu_0 \Delta H$ (b) as function of frequency $f$ for temperatures above and below the superconducting transition.

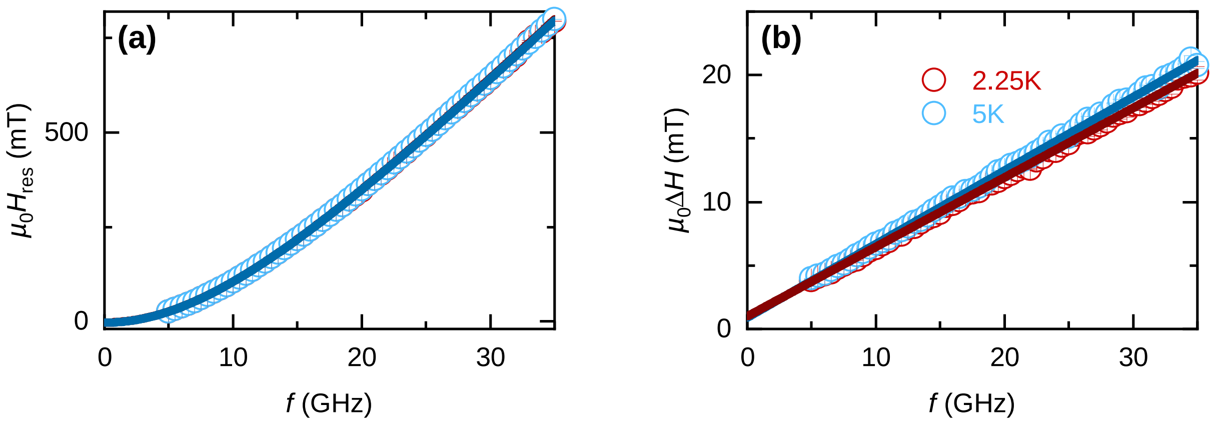


Figure S6. Resonance-field $\mu_0 H_{\rm res}$ (a) and resonance linewidth $\mu_0 \Delta H$ (b) as function of frequency $f$ of sample A for temperatures above ($T = 5$ K) and below $T_{\rm c}$ ($T = 2.25$ K). The lines represent fits to Eq. (S5) for panel (a) and Eq. (S6) for panel (b).

The resonance field $\mu_0 H_{\rm res}$ in Fig. S6(a) is fitted with

$$\mu_0 H_{\rm res} = -\mu_0 H_{\rm ani} - \frac{\mu_0 M_{\rm eff}}{2} + \sqrt{\left(\frac{\mu_0 M_{\rm eff}}{2}\right)^2 + \left(\frac{2\pi f}{\gamma}\right)^2}, \tag{S5}$$

to extract the effective $g$-factor, effective magnetization $\mu_0 M_{\rm eff}$ and in-plane anisotropy $\mu_0 H_{\rm ani}$.

The FMR linewidth $\mu_0 \Delta H(f)$ in Fig. S6(b) is fitted linearly with

$$\mu_0 \Delta H(f) = \mu_0 H_{\rm inh} + 2 \cdot \frac{2\pi f \alpha}{\gamma}. \tag{S6}$$

To extract $\alpha$, we first fit $\mu_0 H_{\rm res}(f)$ to Eq. (S5) and then use the extracted $\gamma$ when fitting $\Delta H(f)$ to Eq. (S6). The inhomogeneous linewidth $\mu_0 \Delta H_{\rm inh}$ is the $f = 0$ Hz offset of the linear fit to Eq. (S6).

In the main text, we illustrated the changes in Gilbert damping $\alpha$ of our TaN/Py sample in the superconducting state. Here we also show the full temperature range from $T \ll T_c$ to RT of the raw magnetization dynamics parameters ($g$-factor, $M_{\mathrm{eff}}$, $H_{\mathrm{ani}}$ and $H_{\mathrm{inh}}$).

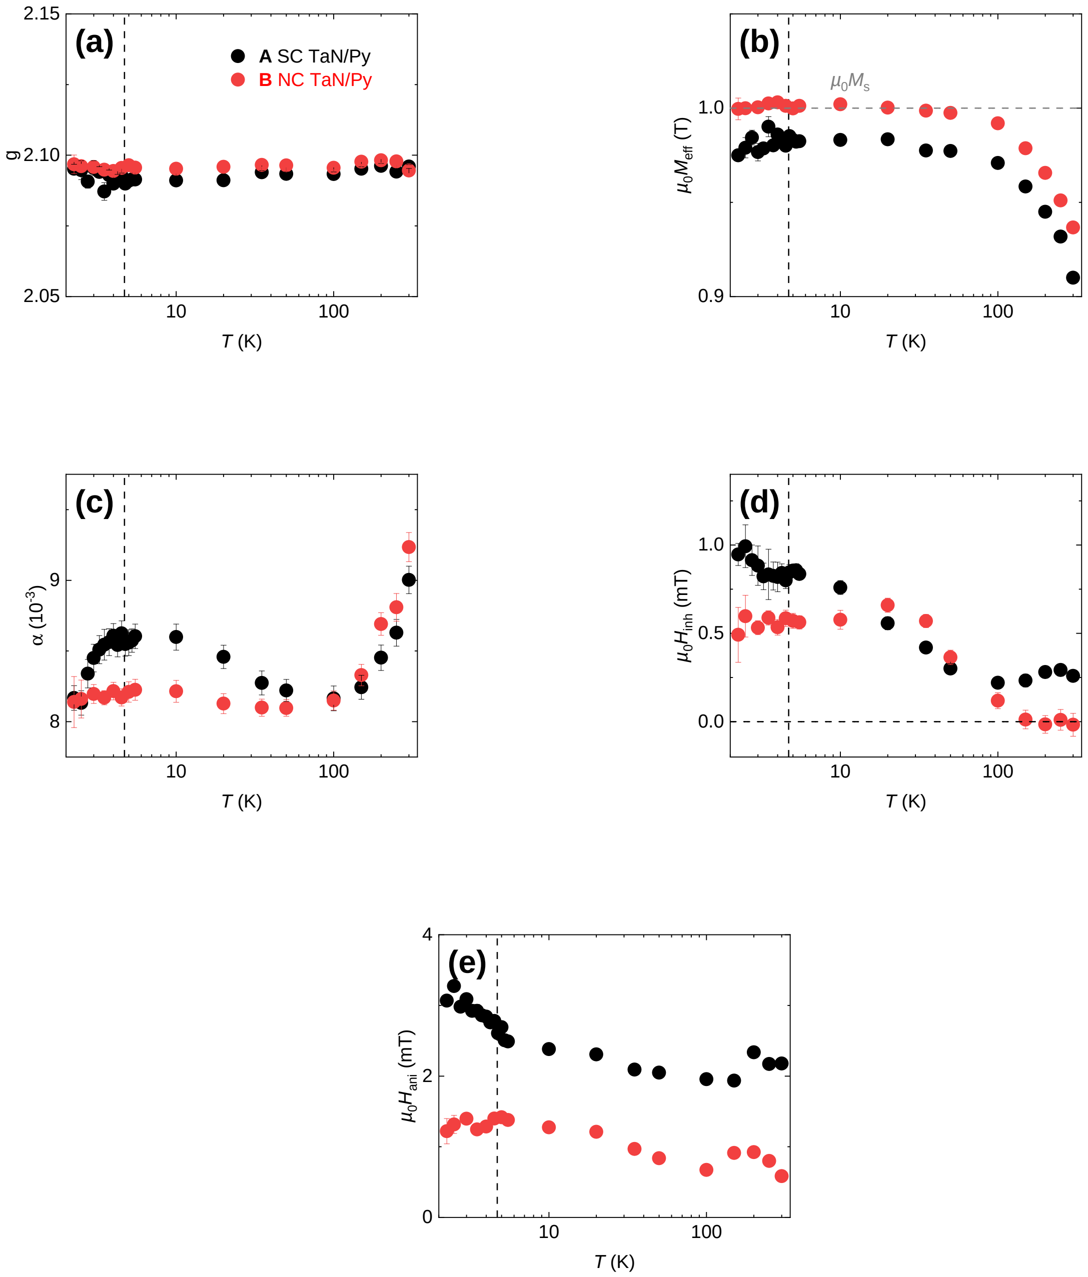


Figure S7. Temperature dependence of spectroscopic parameters of the TaN/Py-sample. (a) The $g$-factor displays no clear dependence on $T$, while the effective magnetization $\mu_0 M_{\mathrm{eff}}$ decreases for increasing temperature due to the thermal excitation of magnons. (c) and (d) illustrate the changes of the Gilbert damping $\alpha$ and inhomogeneous broadening $\mu_0 H_{\mathrm{inh}}$, respectively. (e), The extracted anisotropy field $\mu_0 H_{\mathrm{ani}}$ as function of $T$.

As evident from Fig. S7(a), the $g$-factor exhibits no strong temperature dependence. The effective magnetization $\mu_0 M_{\mathrm{eff}}$ in Fig. S7(b) increases with decreasing $T$, which we attribute to the increase in saturation magnetization with decreasing temperature. The observed temperature dependence of the Gilbert damping $\alpha$ in Fig. S7(c) in the normal state matches previous results[3]. The reduction of $\alpha$ below $T_c$ is due to altered spin transport properties of SC as discussed in the main text. For $\mu_0 H_{\mathrm{inh}}$ in Fig. S7(d) we detect the manifestation of a sizable $\mu_0 H_{\mathrm{inh}}$ for

temperatures slightly above $T_c$. Overall the spectroscopic parameters of Py exhibit only minor changes with $T$ in the normalconducting (NC) state. We observe a small in-plane anisotropy field $\mu_0 H_{ani}$, that gradually rises in the SC state in sample A due to an additional field from SC Meißner currents[5,6].

## VI. RAW DATA FOR THE NORMALIZED INDUCTANCE

From the extracted FMR-amplitude $A$ and $\phi$ from the fitting curve to Fig. S5, we can determine the complex normalized inductance $\tilde{L}(f)$ for all frequencies $f$ using[3,4]

$$\tilde{L} = \frac{1}{\mu_0 M_s} \frac{A e^{i\phi}}{C_0 + C_1 H_{ext}} \frac{Z_0}{\pi f}, \tag{S7}$$

where $Z_0$ =50 Ω is the impedance of the unloaded CPW and $\tilde{L}$ is the normalized inductance $\tilde{L} = L/[\chi_{yy}(f, H_{ext}) + \chi_{zz}(f, H_{ext})]$.
The resulting $\tilde{L}$ of sample A for three selected temperatures, one for $T > T_c$ ($T = 5$ K) and two in the SC state ($T = 3$ K & $T = 2.25$ K), are shown in Fig. S8 in real (a) and imaginary part (b).

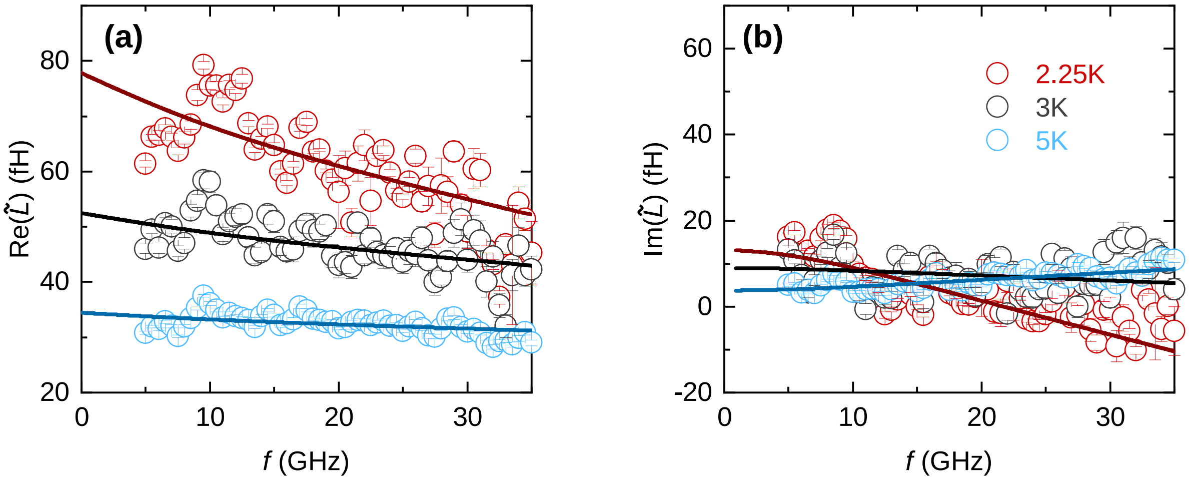


Figure S8. Real (a) and imaginary (b) part of the inductive coupling $\tilde{L}(f)$ as a function of frequency $f$ in the vicinity of $T_c$ ($T = 5$ K and $T = 3$ K) and for $T \ll T_c$ ($T = 2.25$ K). The lines represent fitting curves following Eq. (S8).

We fit $\tilde{L}(f)$ with Eq. (S8), which is derived in our previous publication[3], to extract $\sigma_d$ and $\sigma_f$.

$$\tilde{L} = \begin{cases} \tilde{L}_0^{SC} + i \cdot \tilde{L}_F + 2 \cdot C \cdot \sqrt{\tilde{L}_0^{SC}/\tilde{L}_0} \cdot f \cdot [-\epsilon_r(f)\sigma_f + i\epsilon_i(f)\sigma_d] \,, & \text{for } T \leq T_c \\ \tilde{L}_0 + 2 \cdot C \cdot f \cdot [-\epsilon_r(f)\sigma_f + i\epsilon_i(f)\sigma_d] \,, & \text{for } T > T_c. \end{cases} \tag{S8}$$

Here $\tilde{L}_0^{SC}$ and $\tilde{L}_0$ denote the $f \to 0$ Hz-offset of Re$(\tilde{L})(f)$ in the superconducting and normal state, respectively. $\tilde{L}_F$ represents an offset in the imaginary part from Faraday currents in the SC state, whereas $C$ is a proportionality constant. The functions $\epsilon_r(f)$ and $\epsilon_i(f)$ account for the ellipticity of the magnetization precession cone in the in-plane geometry. All of these expressions are defined in our previous work[3].
We chose to include three temperatures in Fig. S8, to highlight, that the double SC-transition in sample A, that is proposed in the main manuscript, can also clearly be observed in the raw data for $\tilde{L}$. In Fig. S8(a), the rise in slope of the quasi-linear fit with decreasing $T$ highlights the manifestation of the unexpected positive $\sigma_f$ in the SC state. From the imaginary part of $\tilde{L}$ in Fig. S8(b), the sign change of the slope from positive to negative polarity corresponds to the proposed manifestation of the QMiSHE in $\sigma_d$ in the SC state.

## VII. EVIDENCE OF THE SECOND SC TRANSITION AT T=2.5 K

In Fig. S9, we plot the enhancement of the offset of the real part of the normalized inductive coupling between sample and CPW $\tilde{L}_0$, which is a measure of the net CPW driving field $\mathbf{h}_{\mathrm{rf}}$ felt by the FM layer[4], as a function of temperature.

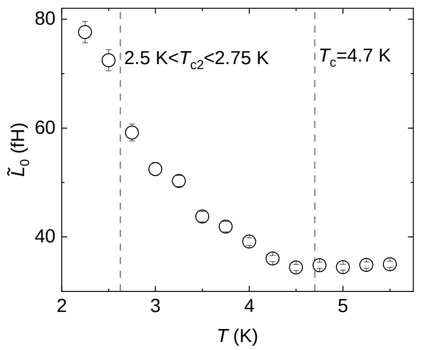


Figure S9. Offset of the real part of the normalized inductive coupling between sample and CPW $\tilde{L}_0$ as a function of temperature $T$. In the SC state, Meißner currents mirror the net oscillatory driving field $\mathbf{h}_{\mathrm{rf}}$ of the CPW. A second SC transition at $(2.5 < T < 2.75)$ K becomes apparent in the abrupt further enhancement of $\tilde{L}_0$

In the SC state, we observe an enhancement in $\tilde{L}_0$ from SC Meißner currents mirroring the CPW driving field. We observe an abrupt further enhancement in $\tilde{L}_0$ for $T < 2.75$ K, attributed to the additional contribution of image currents by the fraction of TaN, which is in direct contact to the FM layer. Hence, we can infer a second SC transition of the TaN thin film from the abrupt change in $\tilde{L}_0$.

## REFERENCES


[1] S. Chaudhuri, I. J. Maasilta, L. Chandernagor, M. Ging, and M. Lahtinen, "Fabrication of superconducting tantalum nitride thin films using infrared pulsed laser deposition," J. Vac. Sci. Technol. A **31**, 061502 (2013).

[2] T. Hashizume, A. Saiki, and K. Terayama, "Fabrication of Tantalum nitride thin film using the low vacuum magnetron sputtering system," IOP conf. ser., Mater. sci. eng. **18**, 14–18 (2011).

[3] M. Müller, L. Liensberger, L. Flacke, H. Huebl, A. Kamra, W. Belzig, R. Gross, M. Weiler, and M. Althammer, "Temperature-dependent spin-transport and current-induced torques in superconductor/ferromagnet heterostructures (Accepted for publication in Physical Review Letters)," arXiv , 1–6 (2020), arXiv:2007.15569.

[4] A. J. Berger, E. R. Edwards, H. T. Nembach, A. D. Karenowska, M. Weiler, and T. J. Silva, "Inductive detection of fieldlike and dampinglike ac inverse spin-orbit torques in ferromagnet/normal-metal bilayers," Phys. Rev. B **97**, 094407 (2018).

[5] K.-R. Jeon, C. Ciccarelli, H. Kurebayashi, L. F. Cohen, X. Montiel, M. Eschrig, T. Wagner, S. Komori, A. Srivastava, J. W. Robinson, and M. G. Blamire, "Effect of Meissner Screening and Trapped Magnetic Flux on Magnetization Dynamics in Thick Nb / $Ni_{80}Fe_{20}$/ Nb Trilayers," Phys. Rev. Appl. , 014061 (2019).

[6] I. Golovchanskiy, N. Abramov, V. Stolyarov, V. Chichkov, M. Silaev, I. Shchetinin, A. Golubov, V. Ryazanov, A. Ustinov, and M. Kupriyanov, "Magnetization Dynamics in Proximity-Coupled Superconductor-Ferromagnet-Superconductor Multilayers," Phys. Rev. Appl. **14**, 024086 (2020).
